# Supplementary material for: On Occlusions in Video Action Detection: Benchmark Datasets And Training Recipes
Source: arXiv:2410.19553 source file (2026-07-10)
Supplement: Supplementary file 1 [file sota.tex]

\subsection{A Robust Video-Level State Of The Art}
\label{sec:sota}
We present a new state-of-the-art in spatio-temporal video action detection specifically on UCF-24 and JHMDB-21 datasets in Tab\ref{tab:sota}. Note that we achieve 83.1\% on UCF-24 and 98.1\% on JHMDB-21 in terms of the widely accepted\cite{kalogeiton2017action} v-mAP metric at the 0.5ioU threshold. One of the most desirable properties in an action-detector is that it should perform well on \textit{existing} standard datasets\cite{soomro2012ucf101} as well as be \textit{robust to occlusions} at the same time. Our simple model namely VCAPS-Mvitv2 achieves the best of both worlds, thereby setting a new video-level state of the art for our community.

The robustness of an action-detector can be measured in two ways, 1) the \textit{actual robustness} under occlusions which has been illustrated  as absolute value (i.e. 67.3\%) in Tab6 of our original manuscript. 2) Measuring the drop in performance of a detector as the ioU threshold during evaluation is swept from $0.2$ to $0.5$. We define this quantity as $\kappa = 1- (\frac{vmAP_{0.2}- vmAP_{0.5}}{vmAP_{0.2}})$ which simply measures the relative performance drop from 0.2$\rightarrow$0.5ioU. In Tab\ref{tab:sota}, we note that on the much challenging UCF-24 dataset, our method obtains $\kappa= 0.84$, which is greater than all the other methods, thereby indicating more localization robustness. On JHMDB-21, we obtain 92.8\% in terms of the absolute v-mAP score, which is significantly better than other existing methods. We acknowledge that TubeR\cite{zhao2022tuber} and ST-Mixer \cite{wu2023stmixer} are slightly better than our method in terms of f-mAP scores on UCF-24 dataset, although our method is considerably \textit{more} robust (0.84 vs 0.71 on $\kappa$ score).

\begin{table}[!htbp]
\caption{\textbf{Comparison with existing methods:} Comparison of our method across existing supervised approaches, *: denotes results using a CSN152 backbone. $\kappa = 1- (\frac{vmAP_{0.2}- vmAP_{0.5}}{vmAP_{0.2}})$. Higher value of $\kappa$ denotes more robustness.}. 
\vspace{-0.4em}
\begin{center}
\begin{tabular}{c|cc|cccc|cccc}
                        &               &              & \multicolumn{4}{c|}{UCF-24}                                    & \multicolumn{4}{c}{JHMDB-21}                                  \\
\midrule
                        & \multicolumn{2}{c|}{Backbone} & f-mAP         & \multicolumn{2}{c}{v-mAP}     &        & f-mAP         & \multicolumn{2}{c}{v-mAP}     &         \\
       Methods                 & 2D            & 3D           & 0.5           & 0.2           & 0.5           &     $\kappa$           & 0.5           & 0.2           & 0.5           &      $\kappa$          \\
\midrule
\textit{Yang et al.}\cite{kalogeiton17iccv}             &     \checkmark          &              & 75.0          & 76.6          & -             & -             & -             & -             & -             & -             \\
\textit{Li et al.}\cite{li2020actions}      &    \checkmark              &              & 78.0          & 82.8          & 53.8          & 0.65          & 70.8          & 77.3          & 70.2          & 0.91          \\
\textit{Kopuklu et al.}\cite{kopuklu2019you} &      \checkmark            &      \checkmark           & 80.4          & 75.8          & 48.8          & 0.64          & 75.7          & 88.3          & 85.9          & 0.97          \\
\textit{Zhao et al.}\cite{zhao2022tuber}    &               &       \checkmark          & \textbf{81.3} & 85.3          & 60.2          & 0.71          & 82.3*         & 81.8          & 80.7          & \textbf{0.99} \\
\textit{Duarte et al.}\cite{duarte2018videocapsulenet}  &               &      \checkmark           & 78.6          & 97.1          & 80.3          & 0.83          & 64.6          & 95.1          & -             & -             \\
\textit{Kumar et al.}\cite{kumar2022end}   &               &     \checkmark            & 69.2          & 95.3          & 71.9          & 0.75          & 68.1          & 96.8          & 68.4          & 0.71          \\
\textit{Tao et al.}\cite{wu2023stmixer}     &               &       \checkmark          & \textbf{83.7} & -             & -             & -             & 86.7          & -             & -             & -             \\
\midrule
\textit{Ours}           &               &    \checkmark             & 81.2          & \textbf{98.6} & \textbf{83.1} & \textbf{0.84} & \textbf{93.0} & \textbf{98.1} & \textbf{92.8} & 0.95         \\
\bottomrule
\end{tabular}
\label{tab:sota}

\end{center} 
\vspace{-1em}
\end{table}
