# Supplementary material for: On Occlusions in Video Action Detection: Benchmark Datasets And Training Recipes
Source: arXiv:2410.19553 source file (2026-07-10)
Supplement: Supplementary file 5 [file intro.tex]

\section{Introduction}
